# Supplementary material for: Heat transfer across a vacuum gap induced by piezoelectrically mediated acoustic phonon tunneling
Source: arXiv:2303.05084 source file (2023-03-09)
Supplement: Supplementary file 1 [file supplementary.pdf]

# Supplementary material: Heat transfer across a vacuum gap induced by piezoelectrically mediated acoustic phonon tunneling

Zhuoran Geng, Ilari J. Maasilta

March 9, 2023

## 1 Crystal orientation

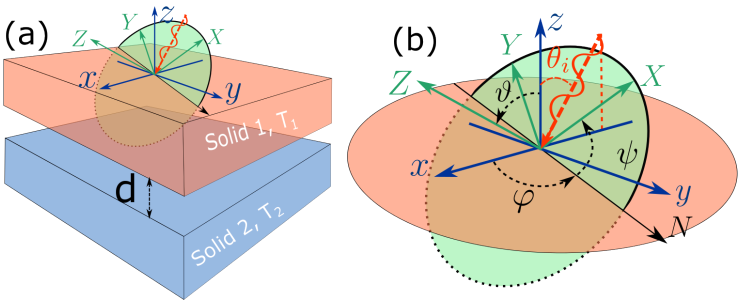


Figure 1: A schematic of the laboratory coordinates $xyz$ and the orientation of the crystal intrinsic coordinates $XYZ$. (a) shows the general layout of the vacuum separated piezoelectric solids 1 and 2, with the two coordinate frames illustrated for solid 1. (b) shows the details of the rotation angles for the crystals and the incident angle of the phonon (red). The orientation of the crystals is signified by a set of Euler angles $(\vartheta, \varphi, \psi)$. An incoming acoustic phonon (red) has a zenith angle $\theta$ and an azimuth angle $\varphi$.

In this work, crystal orientation is described using the Euler angle system with respect to a fixed laboratory coordinate system, the same as in Ref.[1]. In this system, as illustrated in Fig.1, a set of Cartesian laboratory coordinates $xyz$ (blue axes) is chosen to describe the spatial position, whereas a set of orthogonal $XYZ$ coordinates (green axes) is chosen to describe the intrinsic crystal coordinates. The relation between these two frames can be fully expressed by three angles: $\vartheta$, $\varphi$, and $\psi$ as illustrated in panel (b) of Fig.1.

It is particularly important to note here that for the case of a semi-infinite half-space solid, the rotation of the azimuth angle $\varphi$ of the crystal is in fact equivalent to a rotation of the phonon incident azimuth angle, both signifying

the same rotational degree of freedom. Therefore, the rotation of $\varphi$ should only be taken into account once in the mathematical formulation to avoid duplication. For example, we can describe the crystal orientation using only the angles $\vartheta$ and $\psi$, and use $\theta$ and $\varphi$ to describe the incident angle of the phonon.

The formulation presented in the main text takes the material tensors, such as the elastic stiffness tensor $\boldsymbol{c}^E$, the piezoelectric strain tensor $\boldsymbol{e}$, and the electric permittivity tensor $\boldsymbol{\epsilon}^S$, after the rotation transformation by three angles ($\vartheta$, $\psi$ and $\varphi$). The details of the crystal rotation procedures and the transformation of the material tensors have been introduced and explained in Ref.[1].

It is also worth to note that the material tensors will not change with the rotation $\psi$ about the crystal $Z$-axis for a crystal with uniaxial symmetry, which is the case for ZnO and AlN used as example materials in the main article. As a result, the crystal orientation can be simplified further to only a single rotation angle $\vartheta$.

## 2 Group velocity in Stroh-formalism

In piezoelectric solids, the direction of the phonon group velocity doesn't align with that of the phase velocity in general. For a non-dissipative medium, phonon group velocity is identical to the energy flow velocity, and thereby can be obtained from the ratio of the time-averaged acoustic Poynting vector $\boldsymbol{S}$ and the average stored mechanical energy density $(u_K+u_S)/2$, where $u_K$ the peak stored kinetic energy and $u_S$ the peak stored elastic energy [2, 3].

The normal component of the Poynting vector takes the form[1]

$$\hat{\boldsymbol{n}}_\gamma \cdot \boldsymbol{S}_\alpha = \frac{1}{4}\omega_\alpha k \sin\theta |b_\alpha|^2 \hat{\xi}, \tag{1}$$

where for the bulk waves, $\hat{\xi} = \pm 1$ (J/m) is obtained from the Stroh-normalization[4], where the sign determines the direction of the Poynting vector. For bulk waves in an elastic medium, the peak elastic and kinetic stored energies are equal[2] and hence read as

$$(u_S)_\alpha = (u_K)_\alpha = \frac{1}{2}\rho \left| \frac{d\boldsymbol{u}_\alpha}{dt} \right|^2 = \frac{1}{2}\rho\omega_\alpha^2 |b_\alpha|^2 |\boldsymbol{A}_\alpha|^2, \tag{2}$$

where $\rho$ is the density of the solid. As a result, the normal component of the group velocity can be expressed as:

$$\hat{\boldsymbol{n}}_\gamma \cdot \frac{\partial \omega_\alpha}{\partial \boldsymbol{k}} = \frac{\hat{\boldsymbol{n}}_\gamma \cdot \boldsymbol{S}_\alpha}{\frac{1}{2}(u_K + u_S)} = \frac{1}{2} \frac{\sin\theta}{\rho v_\alpha |\boldsymbol{A}_\alpha|^2} \hat{\xi}, \tag{3}$$

It is worth to mention here that, for an outward normal vector $\hat{\boldsymbol{n}}_\gamma$, a positive value of Eq.(3) indicates that the phonon travels in the direction from the solid towards the vacuum.

## 3 Near field radiative heat transfer

The near field radiative heat transfer (NFRHT) of two closely spaced parallel surfaces separated by a vacuum gap of width $d$ has been very well studied. The associated heat flux between surface 1 with temperature $T_1$ and surface 2 with temperature $T_2$ can be obtained from $J^{\rm rad}_{1\to 2} = J^{\rm rad}_1 - J^{\rm rad}_2$ in which $J^{\rm rad}_i$ reads as[5, 6]

$$J^{\rm rad}_i = \frac{1}{\pi^2}\sum_{\sigma=p,s}\int_0^\infty\int_0^\infty {\rm d}\omega k_\parallel {\rm d}k_\parallel \frac{\hbar\omega}{e^{\hbar\omega/k_B T_i}-1}\frac{{\rm Im}(R_{\sigma 1}){\rm Im}(R_{\sigma 2})e^{-2k_\parallel d}}{|1-R_{\sigma 1}R_{\sigma 2}e^{-2k_\parallel d}|^2}, \quad (4)$$

where $\omega$ is the angular frequency, $k_\parallel$ is the component of $\boldsymbol{k}$-vector parallel to the surface, $T_i$ is the temperature of surface $i = 1, 2$, and $R_{\sigma 1}$ and $R_{\sigma 2}$ are the reflection coefficients of surfaces 1 and 2 for wave mode $\sigma = p, s$. These coefficients are given by

$$R_p = \frac{\epsilon k_\perp - k'_\perp}{\epsilon k_\perp + k'_\perp}, \quad R_s = \frac{k_\perp - k'_\perp}{k_\perp + k'_\perp}, \quad (5)$$

where $\epsilon \equiv \epsilon(\omega)$ is the relative dielectric function of the metal, and $k_\perp$ and $k'_\perp$ are the components of $\boldsymbol{k}$-vectors perpendicular to the surface on the vacuum and material sides, respectively,

$$k_\perp = i\sqrt{k_\parallel^2 - \omega/v_c^2}, \quad k'_\perp = i\sqrt{k_\parallel^2 - \epsilon\omega/v_c^2}, \quad (6)$$

where $v_c$ is the speed of light.

The Drude-model dielectric function of Au takes form[7]

$$\epsilon(\omega) = \epsilon_b - \frac{\omega_p^2}{\omega^2 + i\omega\nu}, \quad (7)$$

where we have used $\epsilon_b = 1$, $\omega_p = 1.71 \times 10^{16}\,{\rm s}^{-1}$, $\nu = 4.05 \times 10^{13}\,{\rm s}^{-1}$.

For the dielectric function of ZnO[8, 9], the vertical and parallel vibrational modes have different transverse-optical (TO) and longitudinal-optical (LO) frequencies. Thereby we have used $\epsilon_i$ for different polarizations to substitute $\epsilon$ in Eqs.(4),(5),(6), which reads as

$$\epsilon_i(\omega) = \epsilon_{\infty,i}\frac{\omega^2_{{\rm LO},i} - \omega^2 - i\omega\gamma_i}{\omega^2_{{\rm TO},i} - \omega^2 - i\omega\gamma_i}, \quad (8)$$

where $i = p, s$ describe the electric field polarization parallel or perpendicular to the crystal $Z$-axis, $\gamma_p = \gamma_s = 13\,{\rm cm}^{-1}$ is the damping parameter, and the rest of the parameters are given in Table 1:

## 4 Heat transfer mediated by other phonon tunneling mechanisms

Two other phonon tunneling mechanisms are discussed in the main text: coupling mediated by the van der Waals force and the electrostatic force. The heat

| | $i=p$ | $i=s$ |
|---|---|---|
| $\epsilon_{\infty,i}$ | 3.78 | 3.7 |
| $\omega_{\mathrm{LO},i}$ [cm$^{-1}$] | 574 | 589 |
| $\omega_{\mathrm{TO},i}$ [cm$^{-1}$] | 384 | 411 |

Table 1: Parameters for the dielectric function of ZnO.

flux mediated by these mechanisms can be expressed in a general form developed by Volokitin[10] and given by

$$J_i^{\mathrm{Ph}} = \frac{1}{\pi^2}\int_0^\infty \mathrm{d}\omega \frac{\hbar\omega}{\exp(\hbar\omega/k_B T_i)-1} \times \int_0^\infty \mathrm{d}k_\parallel\, k_\parallel \frac{b^2 \mathrm{Im}M_1 \mathrm{Im}M_2}{|(1-aM_1)(1-aM_2)-b^2M_1M_2|^2}, \tag{9}$$

in which $a$ and $b$ parametrize the coupling mechanism and are defined as

$$\sigma_1 = au_1 - bu_2, \quad \sigma_2 = au_2 - bu_1, \tag{10}$$

where $\sigma_i$ and $u_i$ are the stress and displacement on surface $i = 1, 2$; $M$ is the susceptibility of the material, $u = M\sigma$, and can be obtained as

$$M = \frac{i}{\rho c_t^2}\left(\frac{\omega}{c_t}\right)^2 \frac{p_l}{S}, \tag{11}$$

where

$$S = \left[\left(\frac{\omega}{c_t}\right)^2 - 2k_\parallel^2\right]^2 + 4k_\parallel^2 p_t p_l \qquad p_t = \sqrt{\left(\frac{\omega}{c_t}\right)^2 - k_\parallel^2}, \quad p_l = \sqrt{\left(\frac{\omega}{c_l}\right)^2 - k_\parallel^2}, \tag{12}$$

in which $\rho$, $c_t$, and $c_l$ are the material density, the transverse phase velocity, and the longitudinal phase velocity, respectively.

For the van der Waals interaction, $a$ and $b$ read as

$$a = \frac{H}{2\pi d^4}, \quad b = \frac{H k_\parallel^2 K_2(k_\parallel d)}{4\pi d^2}, \tag{13}$$

where $H$ is the Hamaker constant and $K_2(x)$ is the modified Bessel function of the second kind and second order. We note that by inserting Eqs.(13) into Eq.(9), we confirm that it becomes identical with Eq.(41) in Ref.[6].

With an electrostatic potential difference $V$ between the surfaces, $a$ and $b$ take the form [10]

$$a = \frac{\epsilon_0 V^2 k_\parallel}{d^2}\frac{e^{k_\parallel d} + e^{-k_\parallel d}}{e^{k_\parallel d} - e^{-k_\parallel d}}, \quad b = \frac{\epsilon_0 V^2}{d^2}\frac{2k_\parallel}{e^{k_\parallel d} - e^{-k_\parallel d}}, \tag{14}$$

where we give the equations in SI units, unlike in the original work [10, 11] which uses CGS units.

For acoustic phonon tunneling between two Au surfaces, we use the following parameter values: $\rho = 1.92 \times 10^4\,\mathrm{kgm^{-3}}$, $c_t = 1200\,\mathrm{ms^{-1}}$, $c_l = 3240\,\mathrm{ms^{-1}}$, and $H = 34.7 \times 10^{-20}\,\mathrm{J}$[10].

# 5 Comparing ZnO and AlN with $LiNbO_3$

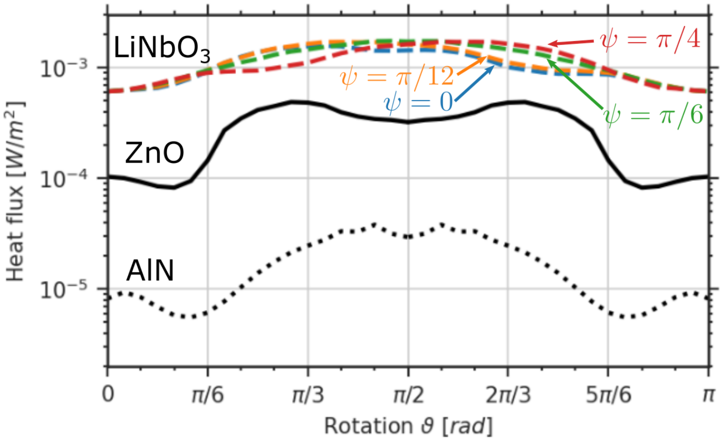


Figure 2: Comparison of emitted PEMHT as a function of the crystal rotation angle $\vartheta$ for ZnO (solid line), AlN (dotted line) and $LiNbO_3$ (colored dashed lines). Four different $\psi$ rotations 0 (blue), $\pi/12$ (orange), $\pi/6$ (green), and $\pi/4$ (red) are plotted for $LiNbO_3$ as its has no uniaxial crystal symmetry. All heat fluxes are calculated for a gap width of 1 nm at a temperature of 0.1 K.

To add to Fig.4 of the main article, we compare the PEMHT of another piezoelectric material, $LiNbO_3$, with ZnO and AlN as a function of crystal rotation. The piezoelectric material constants adopted in the calculations are

$LiNbO_3$ has a trigonal crystal system without the uniaxial symmetry. Consequently, its PEMHT is expected to change with $\psi$ rotations. We demonstrate the PEMHT of $LiNbO_3$ with four different $\psi$ rotations, $0, \pi/12, \pi/6$, and $/\pi/4$ in Fig.2 as a function of $\vartheta$ rotation. By comparing to the results for ZnO, we find that PEMHT is even stronger for $LiNbO_3$, despite the fact that the phase velocities of these two materials are close. This is explained by $LiNbO_3$ having much larger piezoelectric stress constants $e$, as listed in Table.2, leading to an enhanced piezoelectric response on the solid-vacuum interface.

| | ZnO[2] | AlN[12] | $LiNbO_3$[2] |
|---|---|---|---|
| $c^E$ $(10^{10}Nm^{-2})$ | | | |
| $c_{11}$ | 20.97 | 34.5 | 20.3 |
| $c_{33}$ | 21.09 | 39.5 | 24.5 |
| $c_{44}$ | 4.247 | 11.8 | 6 |
| $c_{66}$ | 4.43 | 11 | 7.5 |
| $c_{12}$ | 12.11 | 12.5 | 5.3 |
| $c_{13}$ | 10.51 | 12 | 7.5 |
| $c_{14}$ | | | 0.9 |
| $e$ $(Cm^{-2})$ | | | |
| $e_{15}$ | -0.48 | -0.48 | 3.7 |
| $e_{22}$ | | | 2.5 |
| $e_{31}$ | -0.573 | -0.58 | 0.2 |
| $e_{33}$ | 1.32 | 1.55 | 1.3 |
| $\epsilon^S$ $(\epsilon_0)$ | | | |
| $\epsilon_{xx}$ | 8.55 | 9.04 | 44 |
| $\epsilon_{zz}$ | 10.2 | 10.7 | 29 |
| Density $\rho$ $(kgm^{-3})$ | 5680 | 3260 | 4700 |
| Crystal class | $6mm$ | $6mm$ | $3m$ |

Table 2: Anisotropic piezoelectric material constants used in the numerical calculations.

# References


[1] Z. Geng and I. J. Maasilta, “Acoustic wave tunneling across a vacuum gap between two piezoelectric crystals with arbitrary symmetry and orientation,” *Phys. Rev. Research*, vol. 4, no. 3, p. 033073, 2022.

[2] B. Auld, *Acoustic fields and waves in solids.* Malabar, Florida: Krieger, second ed., 1990.

[3] V. Laude, A. Reinhardt, and A. Khelif, “Equality of the energy and group velocities of bulk acoustic waves in piezoelectric media,” *IEEE Trans. Ultrason. Ferroelectr. Freq. Control*, vol. 52, no. 10, pp. 1869–1871, 2005.

[4] Z. Geng and I. J. Maasilta, “Complete tunneling of acoustic waves between piezoelectric crystals.” arXiv:2209.08287, 2022.

[5] K. Joulain, J.-P. Mulet, F. Marquier, R. Carminati, and J.-J. Greffet, “Surface electromagnetic waves thermally excited: Radiative heat transfer, coherence properties and Casimir forces revisited in the near field,” *Surf. Sci. Rep.*, vol. 57, pp. 59–112, may 2005.

[6] J. B. Pendry, K. Sasihithlu, and R. V. Craster, “Phonon-assisted heat transfer between vacuum-separated surfaces,” *Phys. Rev. B*, vol. 94, no. 7, p. 075414, 2016.

[7] P.-O. Chapuis, S. Volz, C. Henkel, K. Joulain, and J.-J. Greffet, "Effects of spatial dispersion in near-field radiative heat transfer between two parallel metallic surfaces," *Phys. Rev. B*, vol. 77, p. 035431, jan 2008.

[8] N. Ashkenov, B. N. Mbenkum, C. Bundesmann, V. Riede, M. Lorenz, D. Spemann, E. M. Kaidashev, A. Kasic, M. Schubert, M. Grundmann, G. Wagner, H. Neumann, V. Darakchieva, H. Arwin, and B. Monemar, "Infrared dielectric functions and phonon modes of high-quality ZnO films," *J. Appl. Phys.*, vol. 93, no. 1, pp. 126–133, 2003.

[9] P. Ooi, S. Lee, S. Ng, Z. Hassan, and H. A. Hassan, "Far Infrared Optical Properties of Bulk Wurtzite Zinc Oxide Semiconductor," *J. Mater. Sci. Technol.*, vol. 27, no. 5, pp. 465–470, 2011.

[10] A. I. Volokitin, "Contribution of the acoustic waves to near-field heat transfer," *J. Phys.: Condens. Matter*, vol. 32, no. 21, p. 215001, 2020.

[11] A. I. Volokitin, "Effect of an Electric Field in the Heat Transfer between Metals in the Extreme Near Field," *JETP Lett.*, vol. 109, no. 11, pp. 749–754, 2019.

[12] K. Tsubouch and N. Mikoshiba, "Zero-Temperature-Coefficient SAW Devices on AlN Epitaxial Films," *IEEE Trans. Sonics Ultrason.*, vol. 32, no. 5, pp. 634–644, 1985.
